# Supplementary material for: Adapt Before Comparison: A New Perspective on Cross-Domain Few-Shot Segmentation
Source: arXiv:2402.17614 source file (2024-05-17)
Supplement: Supplementary file 1 [file _supplementary.tex]

\input{_constants}
\cameraready % \review OR \camerareadys

\documentclass[10pt,twocolumn,letterpaper]{article}
\input{cvpr_header}
\usepackage{lipsum}
\myexternaldocument{_main}
\begin{document}

%% TITLE
\title{\paperTitle}
\author{\authSorBlock}
\maketitlesupplementary
%%
% if there are bugs swith tables, please uncomment \usepackage{arydshln} in _macros.tex

\input{12_appendix}

{\small
\bibliographystyle{ieeenat_fullname}
\bibliography{11_references, refs/fsl, refs/fss, refs/cd, refs/cdfss, refs/datasets,
refs/lossterms, refs/seg}
}
\end{document}
